# Supplementary material for: Self-stabilizing Balls & Bins in Batches
Source: arXiv:1603.02188 source file (2016-03-07)
Supplement: Supplementary file 1 [file supplements.tex]

% !TEX TS-program = pdflatexmk
% !TEX encoding = UTF-8 Unicode
% !TEX spellcheck = English (United States)
% !TEX root = main.tex

% NOTE: compile this by uncommenting \intput{…} in the main file.

\clearpage
\todo[inline]{everything from here on will be removed from the final submission}

\section{Removed from 1-Choice Process}

\begin{conjecture}
Fix an arbitrary round $t\geq\log n/(1-\lambda)^2$.
With probability $1-\LDAUomicron{1}$ there is a bin $i$ with $\load_i(t)=\LDAUOmega[small]{\frac{\lambda}{1-\lambda}\log\bigl(\frac{n}{1-\lambda}\bigr)}$.
\end{conjecture}
